# Supplementary material for: Randomly Initialized Subnetworks with Iterative Weight Recycling
Source: arXiv:2303.15953 source file (2023-03-28)
Supplement: Supplementary file 1 [file 00-imagenet.tex]

We train ResNet-50 ImageNet models using Edge-Popup with Weight Recycling as well as Biprop with Weight Recycling.  We choose a prune rate of 80\% in order to test the effects of less parameters. In Table \ref{im}, we include results from previous works: ResNet-50 with Edge-Popup, ResNet-50 with IteRand, and Wide ResNet-50 with Biprop.  These results are taken from the Appendix of their respective papers.  

Our algorithm is trained with a warmup period, where recycling is not performed.  We found that training the subnetwork algorithm for a period prior to recycling weights allowed for better convergence.  We set the warmup period to 30 epochs.  Models are trained for 200 epochs, each with SGD optimization, learning rate 0.1, weight decay 3e-5, momentum 0.875, and label smoothing equal to 0.1. For Weight Recycling, the recycling rate $r$ is set to 0.2 and the $K_{per}$ is equal to 10 epochs, similar to the CIFAR10 models. 

We note several more experiments will be executed on larger models and varying prune rates.  %Our GPU cluster limits us to one 

\vspace{1em}
\begin{table}[h]
\begin{center}

\begin{tabular}{|c c c c c|} 
 \hline
 Algorithm & Weights &Prune Rate & \# Parameters& Accuracy  \\ [0.5ex] 
 \hline
  Dense ResNet50 & Floating-point& -&25,557,032& 76.13 \\ 
  Dense Wide-ResNet50 & Floating-point& -&68,883,240& 78.2 \\
  \hline 
 Edge-Popup (RN50)& Floating-point&70\%&7,667,110& 67.11  \\ 
% \hline 
  IteRand (RN50) & Floating-point&70\%&7,667,110& 69.19  \\ 
   Edge-Popup (RN34)& Floating-point&70\%&6,539,302& ~62.2  \\ 
% \hline 
  IteRand  (RN34)& Floating-point&70\%&6,539,302& ~65.9  \\ 
  \textbf{Edge-Popup + Weight Recycle}  & Floating-point&80\%&5,111,406 &67.71 \\ 
   \hline
    Biprop (Wide-ResNet50) & Binary&80\%& 13,776,648 & 74.03\\
 \textbf{  Biprop + Weight Recycle } & Binary& 80\% &5,111,406& 68.15\\

 \hline
\end{tabular}
\end{center}
    \caption{ImageNet results.  Weight Recycling algorithm is trained with the ResNet-50 architecture. }
    \label{im}
\end{table}
